# Supplementary material for: Anomalous dispersion of microswimmer populations
Source: arXiv:2212.01817 ancillary file (2022-12-04)
Supplement: Supplementary file 1 [file SupplementaryInformation.pdf]

# Supplementary Information

## I. MULTIPLE SCALES ANALYSIS FOR THE LONGITUDINAL DISPERSION COEFFICIENT IN PLANE POISEUILLE FLOW

The governing equation for the probability density of the position $(\mathbf{x})$ and orientation $(\mathbf{p})$ of a microswimmer, $\Omega(\mathbf{x}, \mathbf{p}, t)$, with the swimmer undergoing a combination of a run-and-tumble motion and rotary diffusion, the tumbles being perfectly random, is given by[3]:

$$\frac{\partial \Omega}{\partial t} + \nabla_{\mathbf{x}}[(\mathbf{u} + U_s \mathbf{p})\Omega] + \nabla_p \cdot (\dot{\mathbf{p}}\Omega) - D_r \nabla_p^2 \Omega + \frac{1}{4\pi\tau}[\Omega - \int d\mathbf{p}^{'}\Omega(\mathbf{p}^{'})] = 0. \quad \text{(S1)}$$

The probability density $\Omega$ is convected in physical space both due to intrinsic swimming with speed $U_s$ along the swimmer orientation, and the ambient plane Poiseuille flow defined by $\mathbf{u} = U_m[1-(\frac{z}{H})^2]\mathbf{1}_1$; here, $H$ is the channel half-width with the transverse coordinate $z$ ranging from $-H$ to $H$, and $U_m$ is the maximum speed at the centerline $(z = 0)$. The third term in (S1) denotes the convection of $\Omega$ in orientation space due to rotation by the ambient shear, with the rotation rate given by the Jeffery equation, $\dot{\mathbf{p}} = B[\mathbf{E}\cdot\mathbf{p} - \mathbf{p}(\mathbf{E}:\mathbf{pp})] + \mathbf{W}\cdot\mathbf{p}$, $B = \frac{\kappa^2-1}{\kappa^2+1}$ being the Bretherton constant for the spheroidal swimmers of aspect ratio $\kappa$ examined here; $\mathbf{E} = -z\frac{U_m}{H}(\mathbf{1}_1\mathbf{1}_3 + \mathbf{1}_3\mathbf{1}_1)$ and $\mathbf{W} = -z\frac{U_m}{H}(\mathbf{1}_1\mathbf{1}_3 - \mathbf{1}_3\mathbf{1}_1)$ are the rate-of-strain and vorticity tensors of the ambient plane Poiseuille flow. The final two terms in (S1) denote the relaxation of $\Omega$ to isotropy $(\Omega = \frac{1}{4\pi})$ due to both run-and-tumble dynamics and rotary diffusion.

Using $D_r^{-1}$ as the characteristic time scale, and $H$ and $L$ as the characteristic length scales in the longitudinal and transverse directions, respectively, the resulting non-dimensional kinetic equation is given by:

$$\frac{\partial \Omega}{\partial t} + \Lambda\,(\epsilon\, p_1 + Pe_r u_1)\frac{\partial \Omega}{\partial x} + \epsilon\, p_3 \frac{\partial \Omega}{\partial z} + Pe_r \nabla_p \cdot (\dot{\mathbf{p}}\Omega) - \nabla_p^2 \Omega + \frac{1}{4\pi(\tau D_r)}[\Omega - \int d\mathbf{p}^{'}\Omega(\mathbf{p}^{'})] = 0. \quad \text{(S2)}$$

In (S2), $\epsilon = U_s/(HD_r)$ and $\epsilon\Lambda = U_s/(LD_r)$ denote the swimmer Knudsen numbers for $H$ and $L$ as the choices for the macroscopic scale, with $\Lambda = H/L \ll 1$ denoting the asymptotically small ratio of the characteristic transverse and longitudinal length scales. As indicated in the main manuscript, the magnitude of $L$ is typically determined posteriori since it depends on the scaling of the longitudinal diffusivity, $D_{eff}$, that governs the spread of the swimmer population in the flow direction, and is an outcome of the analysis itself. For the classical scenario involving a passive solute, $D_{eff} \approx Pe^2 D$ for $Pe \gg 1$, $D$ being the bare solute diffusivity, and the requirement of the time scale of $O(L^2/D_{eff})$ characterizing longitudinal diffusion, being asymptotically large compared to the time scale of $O(H^2/D)$ governing transverse diffusion, leads to $L \gg Pe\, H$. Here, $Pe = U_m H/D$ is the usual Peclet number based on the solute translational diffusivity. $Pe_r = U_m/HD_r$ in (S2) is the rotary Peclet number. While $Pe_r/\epsilon$ determines the relative importance of convection due to swimming versus that due to the ambient Poiseuille flow, $Pe_r$ alone governs the relative magnitudes of the deterministic rotation by the imposed shear and stochastic relaxation by a combination of run-and-tumble dynamics and rotary diffusion; $Pe_r \gg 1$ denoting the shear-dominant limit. The Peclet number based on the bare translational diffusivity of the swimmer, $D_t \sim U_s^2/D_r$, is given by $Pe = Pe_r/\epsilon^2$. Finally, the dimensionless parameter $\tau D_r$ governs the relative importance of relaxation due to run-and-tumble motion and rotary dffusion, with $\tau D_r = 0$ corresponding to so-called RTPs (run-and-tumble particles) and $\tau D_r = \infty$ corresponding to ABPs (active Brownian particles), the two dominant classes of microswimmers analyzed in the literature. The latter class of swimmers, where $\Omega$ relaxes due to rotary diffusion alone, is the one considered in the manuscript. The main conclusions, in particular, the onset of the anomalous dispersion regime beyond a threshold $Pe_r$, remain unchanged for finite $\tau D_r$, although the $\kappa$-scaling of this threshold Peclet number does depend on $\tau D_r$ owing to a similar dependence observed for the boundary demarcating the transition from high to low-shear trapping[4].

We now use a multiple scales analysis to describe the evolution of a population of microswimmers, within a wide channel corresponding to $\epsilon \ll 1$, and for long enough times that the longitudinal extent of the population is much greater than its transverse extent of $O(H)$[2, 4]. As mentioned above, an estimate of the time scale governing the long-time longitudinal evolution is typically obtained posteriori based on knowledge of the $Pe_r$-scaling of the longitudinal diffusivity. Note that while the multiple scales analysis is restricted to $\epsilon \ll 1$, it remains valid for arbitrary $Pe$ and $Pe_r$. The analysis given below, however, is primarily focused on the limit of large $Pe$ (and $Pe_r$). The hierarchy of temporal evolution regimes has been described in the main manuscript, and is implicit in the following expansion:

$$\Omega(\mathbf{x}, \mathbf{p}, t) = \Omega^{(0)}(x, z, \mathbf{p}, t_1, t_2, t_3; \Lambda) + \epsilon\Omega^{(1)}(x, z, \mathbf{p}, t_1, t_2, t_3; \Lambda) + \epsilon^2\Omega^{(2)}(x, z, \mathbf{p}, t_1, t_2, t_3; \Lambda) + O(\epsilon^3), \quad \text{(S3)}$$

valid for $\epsilon \ll 1$, where $t_1 = t$, $t_2 = \epsilon^2 t$ and $t_3 = \Lambda^2\epsilon^2 t$ correspond to the fast, slow and slower time variables that characterize orientation relaxation, spatial redistribution along the gradient direction, and long-time diffusion along

the flow direction, respectively; note that each of the terms in (S3) depends in addition on $\Lambda$. The dependence on the spanwise coordinate $y$ has been neglected on account of the two-dimensional ambient flow. One may now proceed by directly expanding the time derivative in the form, $\frac{\partial}{\partial t} = \frac{\partial}{\partial t_1} + \epsilon^2 \frac{\partial}{\partial t_2} + \Lambda^2 \epsilon^2 \frac{\partial}{\partial t_3}$ and carrying out the analysis to $O(\epsilon^6)$[2], with the assumption $\Lambda \sim O(\epsilon^2)$ (see below). However, for purposes of clarity, we carry out the multiple scales analysis in two steps. The first step uses the expansion $\frac{\partial}{\partial t} = \frac{\partial}{\partial t_1} + \epsilon^2 \frac{\partial}{\partial t_2}$ as in [4], and leads to a drift-diffusion equation governing the spatial evolution of the microswimmers on the slow time scale $t_2$. In the next step, one uses the expansion $\frac{\partial}{\partial t_2} = \frac{\partial}{\partial t_2} + \Lambda^2 \frac{\partial}{\partial t_3}$, accounting for the separation of the (slow) time scales governing spatial evolution along the gradient and flow directions, respectively. This two-step procedure allows one to conveniently separate the parts of the analysis that involve the orientational and positional degrees of freedom, with the latter component of the analysis bearing a direct connection with the original analysis for a passive solute involving only positional degrees of freedom.

To begin with, using $\frac{\partial}{\partial t} = \frac{\partial}{\partial t_1} + \epsilon^2 \frac{\partial}{\partial t_2}$, one obtains the following equations:

$$\mathcal{O}(1): \frac{\partial \Omega^{(0)}}{\partial t_1} + Pe_r \nabla_p \cdot (\dot{\mathbf{p}} \Omega_0) - \nabla_p^2 \Omega^{(0)} = 0, \tag{S4}$$

$$\mathcal{O}(\epsilon): \frac{\partial \Omega^{(1)}}{\partial t_1} + Pe_r \nabla_p \cdot (\dot{\mathbf{p}} \Omega^{(1)}) - \nabla_p^2 \Omega^{(1)} = -p_3 \frac{\partial \Omega^{(0)}}{\partial z}, \tag{S5}$$

$$\mathcal{O}(\epsilon^2): \frac{\partial \Omega^{(2)}}{\partial t_1} + Pe_r \nabla_p \cdot (\dot{\mathbf{p}} \Omega^{(2)}) - \nabla_p^2 \Omega^{(2)} = -p_3 \frac{\partial \Omega^{(1)}}{\partial z} - (\Lambda/\epsilon^2) Pe_r u_1 \frac{\partial \Omega^{(0)}}{\partial x} - \frac{\partial \Omega^{(0)}}{\partial t_2}. \tag{S6}$$

at successive orders in $\epsilon$ up until $O(\epsilon^2)$. In (S6), we have assumed $\Lambda/\epsilon^2 \sim O(1)$, as a result of which the convective term along $z$ involving swimming alone appears at $O(\epsilon)$, that is in (S5), while the convection along $x$ by the ambient Poiseuille flow appears at $O(\epsilon^2)$. Similar to $L$ above, the above choice of $\Lambda$ may also be justified posteriori; for instance, for $1 \le \kappa \lesssim 2$, one finds $D_{eff} \propto D_t (Pe_r^4/\epsilon^4)$. Using this estimate, and enforcing the separation of longitudinal and transverse evolutions via $L^2/D_{eff} > H^2/D$, one obtains $\Lambda \lesssim \epsilon^2$. We also note that the above choice for $\Lambda$ implies that swimming-induced convection along $x$ appears only at $O(\epsilon^3)$, and therefore, is not included in (S4)-(S6). Thus, the subsequent analysis below, that uses the drift-diffusion equation derived from (S6) as a starting point, is restricted to the limit when convection by the ambient Poiseuille flow is dominant over swimming. This corresponds to $Pe, Pe_r \gg 1$, and accordingly, the expression for the longitudinal diffusivity obtained below is the leading order contribution in the convection-dominant limit. By extending the above analysis to higher orders in $\epsilon$, it may be shown that, among other contributions, the swimming-induced convection along $x$ at $O(\epsilon^3)$ leads to an additional contribution to the longitudinal diffusivity that equals the $z$-averaged bare translational diffusivity $(D_t)$. Hence, in a manner similar to the passive scenario[1], we also include this contribution in the final expression for $D_{eff}$ obtained below, this term being necessary to produce the correct zero-$Pe_r$ asymptote $(D_t)$.

Returning to (S4), the absence of spatial derivatives clearly points to the $\mathbf{x}$ and $\mathbf{p}$ dependencies in $\Omega^{(0)}$ being separable, that is, $\Omega^{(0)} = I(x, z, t_2; \Lambda) G(\mathbf{p}, t_1)$ with $G(\mathbf{p}, t_1)$ for $t_1 \gg 1$ being the quasi-steady orientation distribution commensurate with the local shear rate, achieved for dimensional times much greater than $O(D_r^{-1})$, and the function $I(x, z, t_2; \Lambda)$ characterizing the spatial distribution of the swimmer population along the flow and gradient directions; spatial homogeneity is assumed along the spanwise (vorticity) direction. The orientation distribution $G$ satisfies the equation:

$$Pe_r \nabla_p \cdot (\dot{\mathbf{p}} G) - \nabla_p^2 G = 0, \tag{S7}$$

for large $t_1$, corresponding to a quasi-steady state. Without loss of generality, one may impose the normalization constraint $\int d\mathbf{p} G(\mathbf{p}, t_1) = 1$, so that $\int d\mathbf{p}\, \Omega^{(1)} = \int d\mathbf{p}\, \Omega^{(2)} = 0$ at higher orders. Using the aforementioned separable form for $\Omega^{(0)}$ in (S5), one obtains:

$$\frac{\partial \Omega^{(1)}}{\partial t_1} + Pe_r \nabla_p \cdot (\dot{\mathbf{p}} \Omega^{(1)}) - \nabla_p^2 \Omega^{(1)} = -p_3 G \frac{\partial I}{\partial z} - p_3 \frac{\partial G}{\partial z} I, \tag{S8}$$

where $G$ depends on $z$ via the $z$-dependent shear rate of the plane Poiseuille flow. On account of linearity, one may write $\Omega^{(1)} = \Omega_{11} \frac{\partial I}{\partial z} + \Omega_{12} I$, where $\Omega_{11}$ and $\Omega_{12}$ satisfy equations similar to (S8), but with the individual forcing functions appearing on the RHS; note that the trivial normalization constraint at $O(\epsilon)$ implies $\int d\mathbf{p} \Omega_{11} = \int d\mathbf{p} \Omega_{12} = 0$. Using the above form for $\Omega^{(1)}$ in (S6), and integrating the resulting equation over orientation space leads to the following two-dimensional drift-diffusion equation governing $I$:

$$\frac{\partial I}{\partial t_2} + \Lambda Pe\, u_1 \frac{\partial I}{\partial x} = \frac{\partial}{\partial z} \left( D_{zz} \frac{\partial I}{\partial z} - V_z I \right), \tag{S9}$$

where we have replaced $Pe_r/\epsilon^2$, in the convective term on the LHS, by $Pe$. The drift and diffusion coefficients on the RHS of (S9) are given by:

$$D_{zz}(z; Pe_r, \kappa) = -\int p_3 \Omega_{11}\, d\mathbf{p}, \tag{S10}$$

$$V_z(z; Pe_r, \kappa) = \int p_3 \Omega_{12}\, d\mathbf{p}, \tag{S11}$$

in non-dimensional form, and as indicated by the arguments, are a function of both $Pe_r$ and $\kappa$. As is briefly explained below, it is the dependence on $Pe_r$ that demarcates the different shear-trapping regimes.

Now, treating $\Lambda$ as a small parameter, we write the time derivative in (S9) in the form $\frac{\partial I}{\partial t_2} = \frac{\partial I}{\partial t_2} + \Lambda^2 \frac{\partial I}{\partial t_3}$, while expanding $I$ in a manner analogous to the $\epsilon$-expansion of $\Omega$ above. Prior to doing this, however, it is necessary to transform to a reference frame that moves with the long-time average speed of the swimmer population. Denoting this mean speed as $\bar{u}_1$, defining a new flow coordinate $\bar{x} = x - \bar{u}_1 t_2$, and writing $u_1 = \bar{u}_1 + u_1'$, $u_1'$ being the fluctuating component of the streamwise velocity, (S9) takes the form:

$$\left(\frac{\partial I}{\partial t_2} + \Lambda^2 \frac{\partial I}{\partial t_3}\right) = \frac{\partial}{\partial z}\left(D_{zz}\frac{\partial I}{\partial z} - V_z I\right) - \Lambda Pe\, u_1' \frac{\partial I}{\partial \bar{x}}, \tag{S12}$$

where the mean convection along the flow direction has been subsumed by the new reference frame. The multiple scales expansion of $I$, for small $\Lambda$, may now be written as:

$$I(x, z, t_2, t_3; \Lambda) = I^{(0)}(\bar{x}, z, t_2, t_3) + \Lambda I^{(1)}(\bar{x}, z, t_2, t_3) + \Lambda^2 I^{(2)}(\bar{x}, z, t_2, t_3). \tag{S13}$$

At leading order, one has the following equation governing $I^{(0)}$:

$$\mathcal{O}(1): \frac{\partial I^{(0)}}{\partial t_2} = \frac{\partial}{\partial z}\left(D_{zz}\frac{\partial I^{(0)}}{\partial z} - V_z I^{(0)}\right), \tag{S14}$$

where the absence of $\bar{x}$-derivatives implies a separable dependence on $\bar{x}$ and $z$, so one may write $I^{(0)} = K(\bar{x}, t_3) F(z, t_2)$. Here, $F(z, t_2)$ determines the dependence of the swimmer concentration on the transverse coordinate $z$, evolving on time scales of $O(H^2/D)$, while the amplitude function $K(\bar{x}, t_3)$ governs the spread of the swimmer population in the $x$ direction, for times much greater than $O(H^2/D)$, in a reference frame moving with the mean speed $\bar{u}_1$. For such long times, $F(z, t_2)$ attains a steady state, $F_s(z)$, that satisfies:

$$\frac{d}{dz}\left(D_{zz}\frac{dF_s}{dz} - V_z F_s\right) = 0, \tag{S15}$$

and is therefore given by

$$F_s(z) = \mathcal{N} \exp\left[\int_{-1}^{z} \frac{V_z(z')}{D_{zz}(z')} dz'\right], \tag{S16}$$

where $\mathcal{N}$ is a normalization constant determined from the constraint $\int_{-1}^{1} F_s dz = 1$. Note that this implies $\int_{-1}^{1} I^{(1)} dz = \int_{-1}^{1} I^{(2)} dz = 0$ at $O(\Lambda)$ and $O(\Lambda^2)$, respectively. In [4], the above expression for $F_s$, together with the expressions (S10) and (S11) for the drift ($V_z$) and diffusivity ($D_{zz}$), were derived using a version of the multiple scales analysis used above, but without the amplitude function $K$ above, this being equivalent to assuming the swimmer population to be infinite in extent along the flow direction. The numerical evaluation of the drift and diffusivity expressions, using spherical harmonics expansions for all probability densities involved ($G$, $\Omega_{11}$, $\Omega_{12}$), was then used to understand the high-shear and low-shear trapping regimes, and specifically, the transition from the former to the latter for any finite $\kappa$ with increasing $Pe_r$. It was found that $D_{zz}$ and $V_z$ transition from an $O(Pe_r^{-\frac{4}{3}})$ scaling regime, to an $O(\kappa^2 Pe_r^{-2})$ scaling regime, with increasing $Pe_r$ and for large $\kappa$. This change in scaling is accompanied by a reversal in the drift (a change in sign of $V_z$), from initially pointing wallward to eventually pointing towards the centerline, which leads to the aforementioned change in the trapping regime across a threshold $Pe_r$ of $O(\kappa^3)$.

For the Taylor dispersion problem analyzed here, (S16) serves to define the mean speed which is given by $\bar{u}_1 = \int_{-1}^{1} u_1 F_s(z) dz$; note that $\bar{u}_1 = \frac{2}{3}$ for the classical case of a uniformly distributed passive solute, while for active swimmers with $\kappa \gtrsim 2$, which exhibit a centerline collapse behavior[4], $F_s(z)$ approaches $\delta(z)$ for $Pe_r \to \infty$, so $\bar{u}_1 = 1$

at leading order in this limit. We now derive the equation governing the amplitude function $K(\bar{x}, t_3)$ by considering the governing equations at $O(\Lambda)$ and $O(\Lambda^2)$ which are given by:

$$\mathcal{O}(\Lambda) : \frac{\partial I^{(1)}}{\partial t_2} - \frac{\partial}{\partial z}\left(D_{zz}\frac{\partial I^{(1)}}{\partial z} - V_z I^{(1)}\right) = -\,Pe\,u_1' \frac{\partial I^{(0)}}{\partial \bar{x}}. \tag{S17}$$

$$\mathcal{O}(\Lambda^2) : \frac{\partial I^{(2)}}{\partial t_2} - \frac{\partial}{\partial z}\left(D_{zz}\frac{\partial I^{(2)}}{\partial z} - V_z I^{(2)}\right) = -\,Pe\,u_1' \frac{\partial I^{(1)}}{\partial \bar{x}} - \frac{\partial I^{(0)}}{\partial t_3}. \tag{S18}$$

Substituting the separable form of $I^{(0)}$ above in (S17), one obtains:

$$\mathcal{O}(\Lambda) : \frac{\partial I^{(1)}}{\partial t_2} - \frac{\partial}{\partial z}\left(D_{zz}\frac{\partial I^{(1)}}{\partial z} - V_z I^{(1)}\right) = -Pe u_1' F_s \frac{\partial K}{\partial \bar{x}}. \tag{S19}$$

For large $t_2$, the time derivative in (S19) may be neglected, and (S19) is therefore readily integrated once to yield the following inhomogeneous first order ODE for $I^{(1)}$:

$$\frac{dI^{(1)}}{dz} - \frac{V_z}{D_{zz}} I^{(1)} = Pe \frac{\partial K}{\partial \bar{x}} \frac{1}{D_{zz}(z)} \int_{-1}^{z} u_1'(z') F_s(z') dz', \tag{S20}$$

on using the no-flux condition at the lower channel boundary: $\frac{dI^{(1)}}{dz} - \frac{V_z}{D_{zz}} I^{(1)} = 0$ at $z = -1$. One may solve (S20) using an integrating factor (which is proportional to $F_s^{-1}$), whence one obtains:

$$I^{(1)}(z) = Pe \frac{\partial K}{\partial \bar{x}} F_s(z) \int_{-1}^{z} dz' \frac{1}{F_s(z') D_{zz}(z')} \left(\int_{-1}^{z'} dz'' u_1'(z'') F_s(z'')\right) + J(x) F_s(z). \tag{S21}$$

The above expression already satisfies the no-flux condition at the upper boundary ($z = 1$) regardless of $J(x)$. The latter function may be determined from the normalization constraint (that is, $\int_{-1}^{1} I^{(1)}(z) dz = 0$); importantly, however, the particular expression for $J(x)$ does not affect the expression for $D_{eff}$ obtained below.

Using (S21) in (S18), integrating with respect to $z$ over $[-1, 1]$, and employing the result $\int_{-1}^{1} dz F_s(z) u_1'(z) = 0$, one obtains the following equation governing $K$:

$$\frac{\partial K}{\partial t_3} = \bar{D}_{eff} \frac{\partial^2 K}{\partial \bar{x}^2} \tag{S22}$$

in scaled variables, with

$$\bar{D}_{eff} = -Pe^2 \int_{-1}^{1} dz\, u_1'(z) F_s(z) \int_{-1}^{z} dz' \frac{1}{F_s(z') D_{zz}(z')} \left(\int_{-1}^{z'} dz' u_1'(z'') F_s(z'')\right), \tag{S23}$$

being the leading order approximation to the longitudinal diffusivity in the limit $Pe_r, Pe \gg 1$. One may simplify the integral in (S23) further using an integration by parts, while also using the symmetry of the integrand about the centerline ($z = 0$). This leads to the following simpler expression for the diffusivity:

$$D_{eff} = 2Pe^2 \int_{0}^{1} dz \frac{1}{F_s(z) D_{zz}(z)} \left(\int_{0}^{z} dz' u_1'(z') F_s(z')\right)^2, \tag{S24}$$

which also makes explicit its positive definite character.

On reverting to dimensional variables via $t_3 = \Lambda^2 \epsilon^2 D_r t$ and $x = L\bar{x}$, and going back to the original lab reference frame, the longitudinal length $L$ introduced solely for scaling purposes, cancels out, and (S22) reduces to the convection-diffusion equation:

$$\frac{\partial K}{\partial t} + \bar{u}_1 \frac{\partial H}{\partial x} = D_{eff} \frac{\partial^2 K}{\partial \bar{x}^2} \tag{S25}$$

with the longitudinal diffusivity $D_{eff}$, in dimensional form, being given by

$$D_{eff} = \frac{2U_s^2}{D_r} Pe^2 \int_{0}^{1} dz \frac{1}{F_s(z) D_{zz}(z)} \left(\int_{0}^{z} dz' u_1'(z') F_s(z')\right)^2. \tag{S26}$$

Finally, if one retains the swimming-induced convection along $x$, and goes to the required higher order in $\epsilon$, one obtains an additional contribution to $D_{eff}$, of the form $\int_{-1}^{1} F_s(z)D_{xx}(z)dz$, with $D_{xx}(z; Pe_r, \kappa)$, the flow-aligned component of the swimming-induced diffusion arising from a forcing term of the form $-p_1 G\frac{\partial I}{\partial x}$ at $O(\epsilon^3)$ - this is analogous to what one obtained for $D_{zz}$ above except for $p_3$ being replaced by $p_1$. Adding the dimensional version of this contribution to (S26), one finally obtains the following expression for $D_{eff}$ that is a valid leading order approximation for both $Pe_r \to 0$ and $Pe_r \to \infty$:

$$D_{eff} = \frac{U_s^2}{D_r}\left[\int_{-1}^{1} F_s(z)D_{xx}(z)dz + 2Pe^2\int_0^1 dz\frac{1}{F_s(z)D_{zz}(z)}\left(\int_0^z dz' u_1'(z')F_s(z')\right)^2\right]. \tag{S27}$$

In the limit $Pe_r \to 0$, the first term in (S27), corresponding to the swimming-induced contribution is dominant, and equals unity - this, of course, is to the bare translational diffusivity of the swimmer, $D_t = U_s^2/6D_r$, in the absence of an ambient shearing flow.

For spherical swimmers ($\kappa = 1$), $F_s(z) = \frac{1}{2}$, implying a uniform distribution across the channel similar to a passive solute for any $Pe_r$. Further, it was shown in [4] that the translational diffusivity of a spherical swimmer, although dependent on $Pe_r$, is isotropic, with $D_{zz}(z) = D_{xx}(z) = \frac{2(9+Pe_r^2z^2)}{3(4+Pe_r^2z^2)(9+Pe_r^2z^2)}$. This expression shows the transition of the swimmer diffusivity from its aforementioned quiscent value (1/6) to an $O(Pe_r^{-2})$ scaling for large $Pe_r$, the reduction arising from the rapid rotation-induced decorrelation by the ambient shear, as a result of which the swimmer mean free path decreases from $O(U_s/D_r)$ for $Pe_r \ll 1$ to $O(U_s/D_rPe_4^{-1})$ for $Pe_r \gg 1$. Using these expressions in (S27), one obtains

$$D_{eff} = \frac{U_s^2}{D_r}\left[\frac{1}{3Pe_r}\tan^{-1}\left(\frac{Pe_r}{2}\right) + \frac{Pe_r^2}{\epsilon^4}\left(\frac{16}{315} + \frac{4Pe_r^2}{945}\right)\right], \tag{S28}$$

an expression that is, in fact, valid for arbitrary $Pe_r$ since other contributions may be shown to vanish. For $Pe_r \gg 1$, $\frac{D_{eff}}{U_s^2/D_r} = \frac{4Pe_r^4}{945\epsilon^4}$ - this asymptote, for $\epsilon = 0.1$, appears in Fig 1c of the main manuscript.

## II. NUMERICAL EVALUATION OF THE LONGITUDINAL DISPERSION COEFFICIENT

All of the plots in the main manuscript, including both the concentration profiles and longitudinal diffusivities have been determined from a numerical evaluation of the underlying orientation distributions ($G(\mathbf{p})$, $\Omega_{11}$ and $\Omega_{12}$). In (S7), for instance, the unknown probability density $G(\mathbf{p})$ is expressed as a truncated expansion in spherical harmonics as:

$$G(p) = \sum_{l=0}^{N}\sum_{m=-l}^{l} a_{l,m}Y_l^m(\mathbf{p}), \tag{S29}$$

where $Y_l^m(\mathbf{p}) = \sqrt{\frac{(2l+1)}{4\pi}\frac{(l-m)!}{(l+m)!}}P_l^m(\cos\theta)\exp(im\phi)$ represents the spherical harmonic of order $l$ and degree $m$; $\theta$ and $\phi$ being the polar and azimuthal angles of the spherical coordinate system. Substitution of this expansion, and use of the orthogonality property of the spherical harmonics ($\int d\mathbf{p}Y_l^m(\mathbf{p})Y_{l'}^{m'*}(\mathbf{p}) = \delta_{ll'}\delta_{mm'}$, where $Y_{l'}^{m'*}(\mathbf{p})$ represents the conjugate spherical harmonic), leads to a system of linear equations for the unknown coefficients $a_{l,m}$ ([4]). Along similar lines, using the expansions $\Omega_{11}(p) = \sum_{l=0}^{N}\sum_{m=-l}^{l} b_{l,m}Y_l^m(\mathbf{p})$ and $\Omega_{12}(p) = \sum_{l=0}^{N}\sum_{m=-l}^{l} c_{l,m}Y_l^m(\mathbf{p})$ in (S5), again leads to linear systems that may be solved to obtain $b_{l,m}$ and $c_{l,m}$. The resulting expansions for $\Omega_{11}$ and $\Omega_{12}$ are then used in (S10) and (S11) to calculate $D_{zz}$ and $V_z$. We choose $N = 80$ which ensures the above spherical harmonics expansions converge, in turn leading to converged results for the integrals defining $D_{zz}$ and $V_z$. We evaluate the integral in the expression for the steady state concentration profile $F_s(z)$, given by (S16), using Gauss-Legendre quadrature, taking care to increase the number of quadrature points while also concentrating them in the vicinity of the centerline so as to obtain converged results with increasing $Pe_r$. The integrals involved in $D_{eff}$, as given by (S27), are again evaluated using Gauss-Legendre quadrature, taking particular care to ensure adequate resolution of the shrinking (collapsed) region near the centerline with increasing $Pe_r$. The longitudinal diffusivity results as a function of $Pe_r$, for different $\kappa$, that appear in Fig1c, Fig 2c and Fig 3 of the main manuscript, are obtained using $\epsilon = 0.1$.

---

[S1] Aris, R. On the dispersion of a solute in a fluid flowing through a tube. *Prof. R. Soc. Lond. A235* (1956), 67–77.

[S2] Subramanian, G., and Brady, J. Multiple scales analysis of the fokkerplanck equation for simple shear flow. *Physica A 334*, 3-4 (2004), 343–384.
[S3] Subramanian, G., and Koch, D. L. Critical bacterial concentration for the onset of collective swimming. *Journal of Fluid Mechanics 632* (2009), 359–400.
[S4] Vennamneni, L., Nambiar, S., and Subramanian, G. Shear-induced migration of microswimmers in pressure-driven channel flow. *Journal of Fluid Mechanics 890* (2020).
